# Supplementary material for: Best Axes Composition Extended: Multiple Gyroscopes and Accelerometers Data Fusion to Reduce Systematic Error
Source: arXiv:2209.08895 source file (2022-09-19)
Supplement: Supplementary file 1 [file _07_appendix.tex]

This is used: $\lfp{W}\rf{M} = \lfR{W}\rf{I} \lfp{I}\rf{M} + \lfp{W}\rf{I}$
\begin{align}
    \lf{I_i}\vect{p}\rf{W}(t_k) &= \lf{I_i}\vect{p}\rf{M} - \lfR{I_i}\rf{M}\lfR{M}\rf{W}(t_k) \lf{W}\vect{p}\rf{M}(t_k)\\
    \lf{I_i}\vect{p}^{\scriptscriptstyle GT}\rf{W}(t_k) &= \lf{I_i}\vect{p}\rf{M} - \lfR{I_i}\rf{M}\lfR{M}^{\scriptscriptstyle GT}\rf{W}(t_k) \lf{W}\vect{p}^{\scriptscriptstyle GT}\rf{M}(t_k)
\end{align}

%\begin{equation}
%    \begin{aligned}
%        \lf{M}\vect{a} = 
%        \begin{bmatrix}
%            \lf{I_i} \vect{r}^x \rf{M}\\
%            \lf{I_j} \vect{r}^y \rf{M}\\
%            \lf{I_k} \vect{r}^z \rf{M}
%        \end{bmatrix}^{-1} \left(\rule{0cm}{0.9cm} \begin{bmatrix} \lf{I_i}a^x\\ \lf{I_j}a^y\\ \lf{I_k}a^z \end{bmatrix} + 
%        \begin{bmatrix} 
%            \lf{I_i} a_{inertial}^x\\
%            \lf{I_j} a_{inertial}^y\\
%            \lf{I_k} a_{inertial}^z
%        \end{bmatrix} \right).
%    \end{aligned}
%\end{equation}
